# Supplementary material for: Benchmarking multi-step methods for the dynamic prediction of survival with numerous longitudinal predictors
Source: arXiv:2403.14336 source file (2026-01-13)
Supplement: Supplementary file 1 [file supplementary.pdf]

# Supplementary material for the article: "An empirical appraisal of methods for the dynamic prediction of survival with many longitudinal predictors"

Mirko Signorelli[1] and Sophie Retif[2]

[1]*Mathematical Institute, Leiden University (NL)*
[2]*School of Industrial and Information Engineering, Politecnico di Milano (IT)*

## Contents

**1 Supplementary tables** **1**

**2 Supplementary figures** **11**

## 1 Supplementary tables

| **Variable name** | **Description** | **Variable type** |
|---|---|---|
| ADAS11 | Alzheimer's Disease Assessment Scale (ADAS) 11 | Continuous |
| ADAS13 | ADAS 13 | Continuous |
| ADASQ4 | ADAS Delayed Word Recall | Discrete |
| CDRSB | Clinical Dementia Rating scale Sum of Boxes | Discrete |
| Entorhinal | University of California, San Francisco (UCSF) Entorhinal | Continuous |
| FAQ | FAQ | Discrete |
| Fusiform | UCSF Fusiform | Continuous |
| Hippocampus | UCSF Hippocampus | Continuous |
| ICV | UCSF ICV | Continuous |
| LDELTOTAL | Logical Memory - Delayed Recall | Discrete |
| MidTemp | UCSF Middle temporal gyrus | Continuous |
| MMSE | MMSE | Discrete |
| mPACCdigit | ADNI-modified Preclinical Alzheimer's Cognitive Composite (PACC) with Digit Symbol Substitution | Continuous |
| mPACCtrailsB | ADNI-modified PACC with Trails B | Continuous |
| RAVLT.forgetting | Rey Auditory Verbal Learning Test (RAVLT) Forgetting | Discrete |
| RAVLT.immediate | RAVLT Immediate | Discrete |
| RAVLT.learning | RAVLT Learning | Continuous |
| RAVLT.perc.forgetting | RAVLT Percent Forgetting | Continuous |
| TRABSCOR | Trails B | Continuous |
| Ventricles | UCSF Ventricles | Continuous |
| WholeBrain | UCSF WholeBrain | Continuous |

Table 1: List of longitudinal covariates used as predictors for the ADNI dataset.

| Variable name | Description | Variable type |
|---|---|---|
| bmi | Body mass index | Continuous |
| bradysc | Bradykinesia score | Discrete |
| cesdsum | Depressive symptoms | Discrete |
| cogn_ep | Episodic memory | Continuous |
| cogn_global | Global cognitive function | Continuous |
| cogn_po | Perceptual orientation | Continuous |
| cogn_ps | Perceptual speed | Continuous |
| cogn_se | Semantic memory | Continuous |
| cogn_wo | Working memory | Continuous |
| d_frailty | Frailty | Discrete |
| dbp_avg | Diastolic blood pressure | Continuous |
| gaitsc | Gait score | Continuous |
| iadlsum | Instrumental activities of daily living | Discrete |
| katzsum | Basic activities of daily living | Discrete |
| motor_dexterity | Motor dexterity | Continuous |
| motor_gait | Motor gait | Continuous |
| motor_handstreng | Motor hand strength | Continuous |
| motor10 | Motor function | Continuous |
| parkinsonism_tri | Parkinsonism | Discrete |
| phys5itemsum | Physical activity | Continuous |
| r_depres | Clinical depression | Discrete |
| r_pd | Clinical Parkinson's disease | Discrete |
| r_stroke | Stroke diagnosis | Discrete |
| rigidsc | Rigidity score | Discrete |
| rosbsum | Mobility disability | Discrete |
| sbp_avg | Systolic blood pressure | Continuous |
| soc_net | Social network size | Continuous |
| tremsc | Tremor score | Continuous |
| vasc_risks_sum | Vascular disease risk factors | Continuous |
| vision | Visual acuity | Discrete |

Table 2: List of longitudinal covariates used as predictors for the ROSMAP dataset.

| Variable name | Description | Variable type |
|---|---|---|
| albumin | Albumin | Continuous |
| alkaline | Alkaline phosphatase | Continuous |
| histologic | Histologic stage of disease | Discrete |
| platelets | Platelets | Continuous |
| prothrombin | Prothrombin time | Continuous |
| serBilir | Serum bilirubin | Continuous |
| serChol | Serum cholesterol | Continuous |
| SGOT | Serum glutamic-oxaloacetic transaminase | Continuous |

Table 3: List of longitudinal covariates used as predictors for the PBC2 dataset.

| **Estimation attempt** | **ADNI** | **ROSMAP** | **PBC2** |
|---|---|---|---|
| First | 5 | 15 | 4 |
| Second | 10 | 20 | 6 |
| Third | 15 | 25 | 8 |
| Fourth | 20 | 30 | 10 |

Table 4: Value of $s$ (`nodesize` parameter in the `DynForest` package) used to estimate the trees within the RSFs of DynForest at the first, second, third and fourth estimation attempt.

**Landmark = 2 years**

| Horizon | 3 | 4 | 5 | 6 | 7 | 8 | 9 | 10 |
|---|---|---|---|---|---|---|---|---|
| DynForest | 0.931 | 0.940 | 0.948 | 0.933 | 0.916 | 0.917 | 0.901 | 0.887 |
| FunRSF | 0.923 | 0.924 | 0.930 | 0.915 | 0.892 | 0.893 | 0.885 | 0.848 |
| Landmarking | 0.943 | 0.943 | 0.954 | 0.944 | 0.934 | 0.935 | 0.917 | 0.895 |
| MFPCCox | 0.924 | 0.936 | 0.937 | 0.922 | 0.907 | 0.904 | 0.889 | 0.873 |
| PRC | 0.947 | 0.952 | 0.967 | 0.950 | 0.940 | 0.942 | 0.924 | 0.907 |
| Static Cox | 0.927 | 0.942 | 0.946 | 0.937 | 0.931 | 0.915 | 0.895 | 0.889 |

**Landmark = 3 years**

| Horizon | 4 | 5 | 6 | 7 | 8 | 9 | 10 |
|---|---|---|---|---|---|---|---|
| DynForest | 0.937 | 0.944 | 0.923 | 0.898 | 0.905 | 0.891 | 0.891 |
| FunRSF | 0.927 | 0.934 | 0.905 | 0.884 | 0.878 | 0.872 | 0.831 |
| Landmarking | 0.922 | 0.943 | 0.929 | 0.909 | 0.908 | 0.901 | 0.878 |
| MFPCCox | 0.927 | 0.926 | 0.906 | 0.896 | 0.889 | 0.878 | 0.862 |
| PRC | 0.948 | 0.962 | 0.945 | 0.927 | 0.931 | 0.917 | 0.915 |
| Static Cox | 0.934 | 0.946 | 0.929 | 0.921 | 0.888 | 0.868 | 0.862 |

**Landmark = 4 years**

| Horizon | 5 | 6 | 7 | 8 | 9 | 10 |
|---|---|---|---|---|---|---|
| DynForest | 0.947 | 0.918 | 0.898 | 0.906 | 0.893 | 0.882 |
| FunRSF | 0.939 | 0.920 | 0.889 | 0.884 | 0.872 | 0.834 |
| Landmarking | 0.909 | 0.902 | 0.885 | 0.895 | 0.871 | 0.851 |
| MFPCCox | 0.930 | 0.910 | 0.891 | 0.898 | 0.875 | 0.844 |
| PRC | 0.960 | 0.939 | 0.927 | 0.938 | 0.922 | 0.908 |
| Static Cox | 0.939 | 0.913 | 0.906 | 0.871 | 0.853 | 0.855 |

Table 5: Cross-validation estimates of the time-dependent AUC for the ADNI dataset

**Landmark = 2 years**

| Horizon | 3 | 4 | 5 | 6 | 7 | 8 | 9 | 10 |
|---|---|---|---|---|---|---|---|---|
| DynForest | 0.043 | 0.060 | 0.060 | 0.070 | 0.084 | 0.090 | 0.102 | 0.120 |
| FunRSF | 0.047 | 0.071 | 0.079 | 0.092 | 0.105 | 0.110 | 0.119 | 0.145 |
| Landmarking | 0.042 | 0.059 | 0.061 | 0.070 | 0.079 | 0.083 | 0.093 | 0.114 |
| MFPCCox | 0.046 | 0.062 | 0.068 | 0.077 | 0.089 | 0.093 | 0.102 | 0.124 |
| PRC | 0.041 | 0.056 | 0.053 | 0.062 | 0.072 | 0.076 | 0.088 | 0.106 |
| Static Cox | 0.040 | 0.051 | 0.054 | 0.064 | 0.072 | 0.082 | 0.097 | 0.113 |

**Landmark = 3 years**

| Horizon | 4 | 5 | 6 | 7 | 8 | 9 | 10 |
|---|---|---|---|---|---|---|---|
| DynForest | 0.039 | 0.048 | 0.061 | 0.076 | 0.083 | 0.097 | 0.115 |
| FunRSF | 0.043 | 0.057 | 0.075 | 0.088 | 0.099 | 0.112 | 0.142 |
| Landmarking | 0.041 | 0.049 | 0.060 | 0.073 | 0.080 | 0.090 | 0.109 |
| MFPCCox | 0.042 | 0.052 | 0.066 | 0.080 | 0.087 | 0.101 | 0.122 |
| PRC | 0.041 | 0.044 | 0.056 | 0.069 | 0.074 | 0.086 | 0.102 |
| Static Cox | 0.033 | 0.040 | 0.055 | 0.063 | 0.078 | 0.095 | 0.114 |

**Landmark = 4 years**

| Horizon | 5 | 6 | 7 | 8 | 9 | 10 |
|---|---|---|---|---|---|---|
| DynForest | 0.029 | 0.046 | 0.064 | 0.072 | 0.086 | 0.108 |
| FunRSF | 0.032 | 0.056 | 0.074 | 0.088 | 0.103 | 0.130 |
| Landmarking | 0.029 | 0.046 | 0.068 | 0.081 | 0.101 | 0.130 |
| MFPCCox | 0.031 | 0.050 | 0.066 | 0.077 | 0.094 | 0.112 |
| PRC | 0.028 | 0.043 | 0.058 | 0.065 | 0.080 | 0.096 |
| Static Cox | 0.022 | 0.046 | 0.055 | 0.076 | 0.093 | 0.112 |

Table 6: Cross-validated Brier score estimates for the ADNI dataset

**Landmark = 2 years**

| Horizon | 3 | 4 | 5 | 6 | 7 | 8 | 9 | 10 | 11 | 12 | 13 | 14 | 15 |
|---|---|---|---|---|---|---|---|---|---|---|---|---|---|
| FunRSF | 0.887 | 0.896 | 0.891 | 0.891 | 0.875 | 0.867 | 0.857 | 0.862 | 0.869 | 0.871 | 0.882 | 0.882 | 0.872 |
| Landmarking | 0.923 | 0.915 | 0.908 | 0.905 | 0.897 | 0.887 | 0.877 | 0.888 | 0.896 | 0.895 | 0.909 | 0.907 | 0.893 |
| MFPCCox | 0.909 | 0.895 | 0.894 | 0.895 | 0.888 | 0.882 | 0.874 | 0.884 | 0.890 | 0.891 | 0.905 | 0.902 | 0.890 |
| PRC | 0.913 | 0.910 | 0.906 | 0.907 | 0.900 | 0.892 | 0.886 | 0.896 | 0.902 | 0.900 | 0.912 | 0.911 | 0.899 |
| Static Cox | 0.869 | 0.867 | 0.876 | 0.887 | 0.874 | 0.859 | 0.861 | 0.870 | 0.877 | 0.876 | 0.896 | 0.903 | 0.902 |

**Landmark = 3 years**

| Horizon | 4 | 5 | 6 | 7 | 8 | 9 | 10 | 11 | 12 | 13 | 14 | 15 |
|---|---|---|---|---|---|---|---|---|---|---|---|---|
| DynForest | 0.933 | 0.937 | 0.931 | 0.908 | 0.900 | 0.891 | 0.896 | 0.900 | 0.899 | 0.908 | 0.900 | 0.888 |
| FunRSF | 0.916 | 0.919 | 0.905 | 0.892 | 0.882 | 0.874 | 0.878 | 0.878 | 0.869 | 0.875 | 0.875 | 0.865 |
| Landmarking | 0.919 | 0.921 | 0.915 | 0.911 | 0.905 | 0.897 | 0.900 | 0.901 | 0.904 | 0.912 | 0.915 | 0.903 |
| MFPCCox | 0.886 | 0.905 | 0.909 | 0.905 | 0.897 | 0.888 | 0.895 | 0.897 | 0.896 | 0.909 | 0.907 | 0.895 |
| PRC | 0.927 | 0.921 | 0.917 | 0.914 | 0.910 | 0.903 | 0.914 | 0.913 | 0.910 | 0.917 | 0.918 | 0.907 |
| Static Cox | 0.845 | 0.861 | 0.877 | 0.858 | 0.843 | 0.846 | 0.859 | 0.870 | 0.869 | 0.890 | 0.897 | 0.898 |

**Landmark = 4 years**

| Horizon | 5 | 6 | 7 | 8 | 9 | 10 | 11 | 12 | 13 | 14 | 15 |
|---|---|---|---|---|---|---|---|---|---|---|---|
| DynForest | 0.930 | 0.922 | 0.921 | 0.915 | 0.906 | 0.906 | 0.903 | 0.899 | 0.909 | 0.923 | 0.908 |
| FunRSF | 0.934 | 0.921 | 0.895 | 0.886 | 0.888 | 0.885 | 0.890 | 0.875 | 0.881 | 0.889 | 0.877 |
| Landmarking | 0.937 | 0.931 | 0.922 | 0.910 | 0.903 | 0.902 | 0.903 | 0.905 | 0.915 | 0.917 | 0.901 |
| MFPCCox | 0.935 | 0.926 | 0.911 | 0.900 | 0.896 | 0.903 | 0.906 | 0.894 | 0.905 | 0.909 | 0.896 |
| PRC | 0.945 | 0.931 | 0.927 | 0.921 | 0.914 | 0.923 | 0.924 | 0.920 | 0.925 | 0.927 | 0.914 |
| Static Cox | 0.865 | 0.879 | 0.853 | 0.836 | 0.840 | 0.853 | 0.864 | 0.870 | 0.890 | 0.898 | 0.903 |

**Landmark = 5 years**

| Horizon | 6 | 7 | 8 | 9 | 10 | 11 | 12 | 13 | 14 | 15 |
|---|---|---|---|---|---|---|---|---|---|---|
| Landmarking | 0.929 | 0.922 | 0.910 | 0.913 | 0.914 | 0.916 | 0.920 | 0.928 | 0.926 | 0.911 |
| PRC | 0.920 | 0.921 | 0.916 | 0.920 | 0.928 | 0.926 | 0.924 | 0.929 | 0.930 | 0.919 |
| Static Cox | 0.878 | 0.825 | 0.813 | 0.822 | 0.839 | 0.852 | 0.860 | 0.882 | 0.891 | 0.898 |

**Landmark = 6 years**

| Horizon | 7 | 8 | 9 | 10 | 11 | 12 | 13 | 14 | 15 |
|---|---|---|---|---|---|---|---|---|---|
| DynForest | 0.935 | 0.921 | 0.929 | 0.930 | 0.930 | 0.930 | 0.929 | 0.927 | 0.907 |
| FunRSF | 0.856 | 0.881 | 0.879 | 0.885 | 0.892 | 0.885 | 0.895 | 0.894 | 0.891 |
| Landmarking | 0.934 | 0.924 | 0.921 | 0.929 | 0.931 | 0.930 | 0.936 | 0.936 | 0.916 |
| MFPCCox | 0.906 | 0.905 | 0.902 | 0.907 | 0.908 | 0.911 | 0.921 | 0.916 | 0.904 |
| PRC | 0.937 | 0.926 | 0.930 | 0.936 | 0.936 | 0.936 | 0.938 | 0.937 | 0.924 |
| Static Cox | 0.803 | 0.794 | 0.810 | 0.830 | 0.847 | 0.861 | 0.881 | 0.885 | 0.892 |

Table 7: Cross-validation estimates of the time-dependent AUC for the ROSMAP dataset

**Landmark = 2 years**

| Horizon | 3 | 4 | 5 | 6 | 7 | 8 | 9 | 10 | 11 | 12 | 13 | 14 | 15 |
|---|---|---|---|---|---|---|---|---|---|---|---|---|---|
| FunRSF | 0.028 | 0.048 | 0.064 | 0.076 | 0.095 | 0.109 | 0.122 | 0.127 | 0.132 | 0.139 | 0.141 | 0.142 | 0.149 |
| Landmarking | 0.027 | 0.044 | 0.060 | 0.068 | 0.084 | 0.096 | 0.108 | 0.110 | 0.114 | 0.120 | 0.118 | 0.120 | 0.129 |
| MFPCCox | 0.028 | 0.045 | 0.061 | 0.069 | 0.085 | 0.097 | 0.109 | 0.110 | 0.114 | 0.120 | 0.119 | 0.122 | 0.130 |
| PRC | 0.027 | 0.045 | 0.060 | 0.068 | 0.081 | 0.092 | 0.104 | 0.105 | 0.110 | 0.117 | 0.116 | 0.117 | 0.123 |
| Static Cox | 0.030 | 0.050 | 0.065 | 0.073 | 0.089 | 0.106 | 0.120 | 0.122 | 0.124 | 0.132 | 0.129 | 0.128 | 0.130 |

**Landmark = 3 years**

| Horizon | 4 | 5 | 6 | 7 | 8 | 9 | 10 | 11 | 12 | 13 | 14 | 15 |
|---|---|---|---|---|---|---|---|---|---|---|---|---|
| DynForest | 0.026 | 0.042 | 0.053 | 0.072 | 0.084 | 0.095 | 0.104 | 0.111 | 0.119 | 0.118 | 0.122 | 0.132 |
| FunRSF | 0.025 | 0.044 | 0.059 | 0.078 | 0.093 | 0.107 | 0.114 | 0.122 | 0.133 | 0.138 | 0.140 | 0.148 |
| Landmarking | 0.025 | 0.042 | 0.052 | 0.071 | 0.083 | 0.095 | 0.099 | 0.106 | 0.111 | 0.114 | 0.113 | 0.122 |
| MFPCCox | 0.025 | 0.044 | 0.053 | 0.071 | 0.083 | 0.097 | 0.100 | 0.108 | 0.114 | 0.115 | 0.118 | 0.126 |
| PRC | 0.024 | 0.042 | 0.053 | 0.068 | 0.079 | 0.092 | 0.093 | 0.102 | 0.109 | 0.110 | 0.109 | 0.117 |
| Static Cox | 0.028 | 0.049 | 0.062 | 0.082 | 0.101 | 0.117 | 0.122 | 0.125 | 0.133 | 0.131 | 0.130 | 0.132 |

**Landmark = 4 years**

| Horizon | 5 | 6 | 7 | 8 | 9 | 10 | 11 | 12 | 13 | 14 | 15 |
|---|---|---|---|---|---|---|---|---|---|---|---|
| DynForest | 0.031 | 0.048 | 0.061 | 0.074 | 0.085 | 0.094 | 0.106 | 0.117 | 0.121 | 0.117 | 0.127 |
| FunRSF | 0.027 | 0.048 | 0.072 | 0.087 | 0.100 | 0.109 | 0.114 | 0.128 | 0.133 | 0.131 | 0.141 |
| Landmarking | 0.025 | 0.039 | 0.058 | 0.075 | 0.088 | 0.094 | 0.101 | 0.110 | 0.111 | 0.111 | 0.122 |
| MFPCCox | 0.030 | 0.042 | 0.063 | 0.074 | 0.085 | 0.090 | 0.097 | 0.113 | 0.114 | 0.112 | 0.123 |
| PRC | 0.024 | 0.038 | 0.057 | 0.069 | 0.083 | 0.086 | 0.093 | 0.102 | 0.105 | 0.104 | 0.113 |
| Static Cox | 0.029 | 0.046 | 0.070 | 0.091 | 0.109 | 0.116 | 0.121 | 0.129 | 0.128 | 0.127 | 0.128 |

**Landmark = 5 years**

| Horizon | 6 | 7 | 8 | 9 | 10 | 11 | 12 | 13 | 14 | 15 |
|---|---|---|---|---|---|---|---|---|---|---|
| Landmarking | 0.024 | 0.049 | 0.067 | 0.078 | 0.085 | 0.092 | 0.098 | 0.100 | 0.103 | 0.113 |
| PRC | 0.022 | 0.048 | 0.061 | 0.073 | 0.078 | 0.087 | 0.097 | 0.100 | 0.101 | 0.108 |
| Static Cox | 0.024 | 0.054 | 0.081 | 0.103 | 0.113 | 0.119 | 0.129 | 0.130 | 0.129 | 0.129 |

**Landmark = 6 years**

| Horizon | 7 | 8 | 9 | 10 | 11 | 12 | 13 | 14 | 15 |
|---|---|---|---|---|---|---|---|---|---|
| DynForest | 0.034 | 0.055 | 0.066 | 0.075 | 0.084 | 0.092 | 0.098 | 0.101 | 0.116 |
| FunRSF | 0.038 | 0.062 | 0.081 | 0.093 | 0.104 | 0.120 | 0.125 | 0.128 | 0.134 |
| Landmarking | 0.035 | 0.054 | 0.068 | 0.075 | 0.081 | 0.089 | 0.092 | 0.094 | 0.106 |
| MFPCCox | 0.034 | 0.053 | 0.071 | 0.078 | 0.089 | 0.100 | 0.102 | 0.106 | 0.113 |
| PRC | 0.033 | 0.048 | 0.063 | 0.069 | 0.078 | 0.087 | 0.092 | 0.094 | 0.103 |
| Static Cox | 0.037 | 0.070 | 0.098 | 0.109 | 0.116 | 0.126 | 0.130 | 0.131 | 0.132 |

Table 8: Cross-validated Brier score estimates for the ROSMAP dataset

**Landmark = 2.5 years**

| Horizon | 3.5 | 4.5 | 5.5 | 6.5 | 7.5 |
|---|---|---|---|---|---|
| DynForest | 0.896 | 0.887 | 0.882 | 0.848 | 0.851 |
| FunRSF | 0.846 | 0.824 | 0.850 | 0.824 | 0.817 |
| Landmarking | 0.922 | 0.886 | 0.865 | 0.829 | 0.838 |
| MFPCCox | 0.859 | 0.819 | 0.828 | 0.788 | 0.786 |
| PRC | 0.903 | 0.900 | 0.906 | 0.874 | 0.870 |
| Static Cox | 0.898 | 0.897 | 0.884 | 0.860 | 0.831 |

**Landmark = 3 years**

| Horizon | 4 | 5 | 6 | 7 | 8 |
|---|---|---|---|---|---|
| DynForest | 0.865 | 0.851 | 0.840 | 0.846 | 0.836 |
| FunRSF | 0.816 | 0.830 | 0.813 | 0.804 | 0.789 |
| Landmarking | 0.860 | 0.855 | 0.833 | 0.846 | 0.836 |
| MFPCCox | 0.828 | 0.861 | 0.846 | 0.857 | 0.836 |
| PRC | 0.866 | 0.887 | 0.872 | 0.882 | 0.860 |
| Static Cox | 0.872 | 0.871 | 0.815 | 0.838 | 0.794 |

**Landmark = 3.5 years**

| Horizon | 4.5 | 5.5 | 6.5 | 7.5 |
|---|---|---|---|---|
| DynForest | 0.839 | 0.859 | 0.838 | 0.840 |
| FunRSF | 0.811 | 0.868 | 0.829 | 0.821 |
| Landmarking | 0.907 | 0.845 | 0.840 | 0.851 |
| MFPCCox | 0.875 | 0.870 | 0.832 | 0.841 |
| PRC | 0.904 | 0.899 | 0.869 | 0.870 |
| Static Cox | 0.888 | 0.862 | 0.824 | 0.803 |

Table 9: Cross-validation estimates of the time-dependent AUC for the PBC2 dataset

**Landmark = 2.5 years**

| Horizon | 3.5 | 4.5 | 5.5 | 6.5 | 7.5 |
|---|---|---|---|---|---|
| DynForest | 0.052 | 0.076 | 0.095 | 0.115 | 0.127 |
| FunRSF | 0.059 | 0.089 | 0.112 | 0.133 | 0.152 |
| Landmarking | 0.046 | 0.074 | 0.094 | 0.115 | 0.120 |
| MFPCCox | 0.062 | 0.094 | 0.113 | 0.138 | 0.154 |
| PRC | 0.054 | 0.076 | 0.091 | 0.109 | 0.114 |
| Static Cox | 0.049 | 0.077 | 0.099 | 0.116 | 0.136 |

**Landmark = 3 years**

| Horizon | 4 | 5 | 6 | 7 | 8 |
|---|---|---|---|---|---|
| DynForest | 0.051 | 0.086 | 0.105 | 0.121 | 0.137 |
| FunRSF | 0.060 | 0.094 | 0.118 | 0.144 | 0.161 |
| Landmarking | 0.051 | 0.092 | 0.105 | 0.113 | 0.129 |
| MFPCCox | 0.065 | 0.090 | 0.103 | 0.118 | 0.131 |
| PRC | 0.051 | 0.083 | 0.099 | 0.108 | 0.127 |
| Static Cox | 0.044 | 0.081 | 0.111 | 0.122 | 0.151 |

**Landmark = 3.5 years**

| Horizon | 4.5 | 5.5 | 6.5 | 7.5 |
|---|---|---|---|---|
| DynForest | 0.047 | 0.082 | 0.104 | 0.120 |
| FunRSF | 0.048 | 0.082 | 0.110 | 0.133 |
| Landmarking | 0.050 | 0.081 | 0.101 | 0.109 |
| MFPCCox | 0.056 | 0.083 | 0.111 | 0.122 |
| PRC | 0.047 | 0.078 | 0.103 | 0.111 |
| Static Cox | 0.045 | 0.084 | 0.110 | 0.137 |

Table 10: Cross-validated Brier score estimates for the PBC2 dataset

| | Landmark | | | |
|---|---|---|---|---|
| Method | 2 | 3 | 4 | Average |
| Static Cox | 0.009 | 0.007 | 0.006 | 0.007 |
| Landmarking | 0.010 | 0.007 | 0.006 | 0.008 |
| MFPCCox | 0.080 | 0.046 | 0.046 | 0.057 |
| PRC | 0.776 | 0.482 | 0.453 | 0.571 |
| FunRSF | 0.240 | 0.122 | 0.125 | 0.163 |
| DynForest | 12.501 | 9.077 | 8.099 | 9.892 |

Table 11: Average computing time per CV fold (in **minutes**) for the ADNI dataset.

| | Landmark | | | | | |
|---|---|---|---|---|---|---|
| Method | 2 | 3 | 4 | 5 | 6 | Average |
| Static Cox | 0.022 | 0.019 | 0.016 | 0.014 | 0.011 | 0.017 |
| Landmarking | 0.023 | 0.020 | 0.017 | 0.014 | 0.011 | 0.017 |
| MFPCCox | 0.194 | 0.135 | 0.066 | - | 0.064 | 0.115 |
| PRC | 3.755 | 1.151 | 1.138 | 1.115 | 1.124 | 1.657 |
| FunRSF | 0.604 | 0.367 | 0.115 | - | 0.124 | 0.302 |
| DynForest | - | 11.504 | 17.657 | - | 34.147 | 21.102 |

Table 12: Average computing time per CV fold (in **minutes**) for the ROSMAP dataset.

| | Landmark | | | |
|---|---|---|---|---|
| Method | 2.5 | 3 | 3.5 | Average |
| Static Cox | 0.253 | 0.246 | 0.177 | 0.226 |
| Landmarking | 0.260 | 0.240 | 0.188 | 0.229 |
| MFPCCox | 0.902 | 0.522 | 0.556 | 0.660 |
| PRC | 7.832 | 7.616 | 7.762 | 7.737 |
| FunRSF | 2.776 | 1.393 | 1.526 | 1.898 |
| DynForest | 186.136 | 136.747 | 128.914 | 150.599 |

Table 13: Average computing time per CV fold (in **seconds**) for the PBC2 dataset.

# 2 Supplementary figures

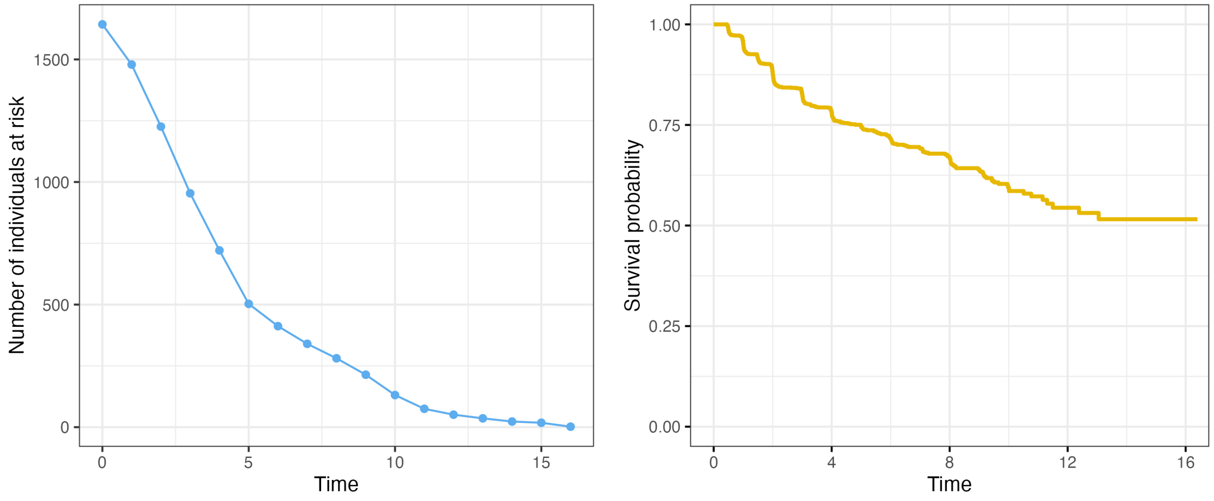


Figure 1: Number of subjects at risk (left) and Kaplan-Meier chart (right) for the ADNI dataset.

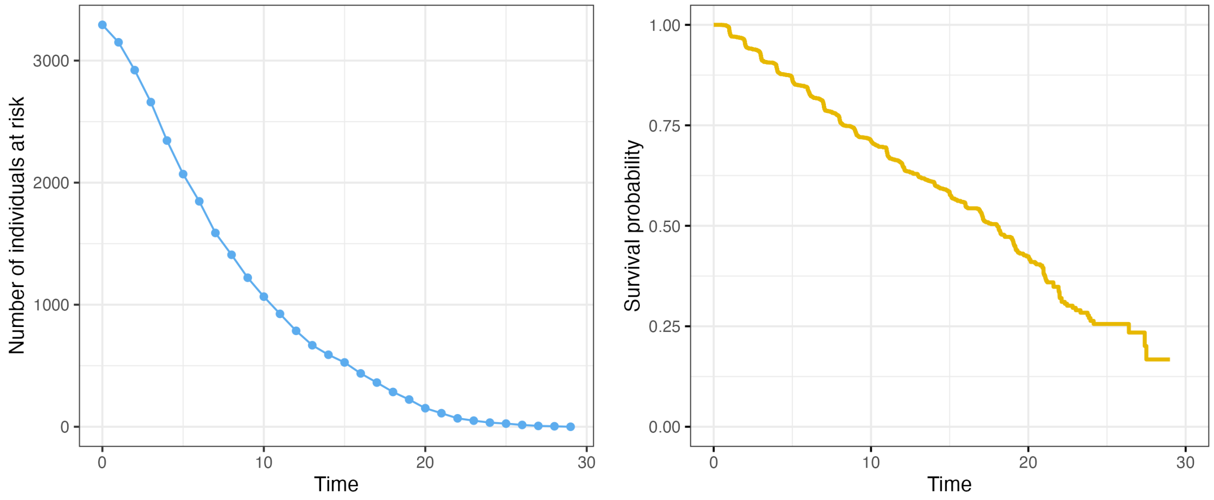


Figure 2: Number of subjects at risk (left) and Kaplan-Meier chart (right) for the ROSMAP dataset.

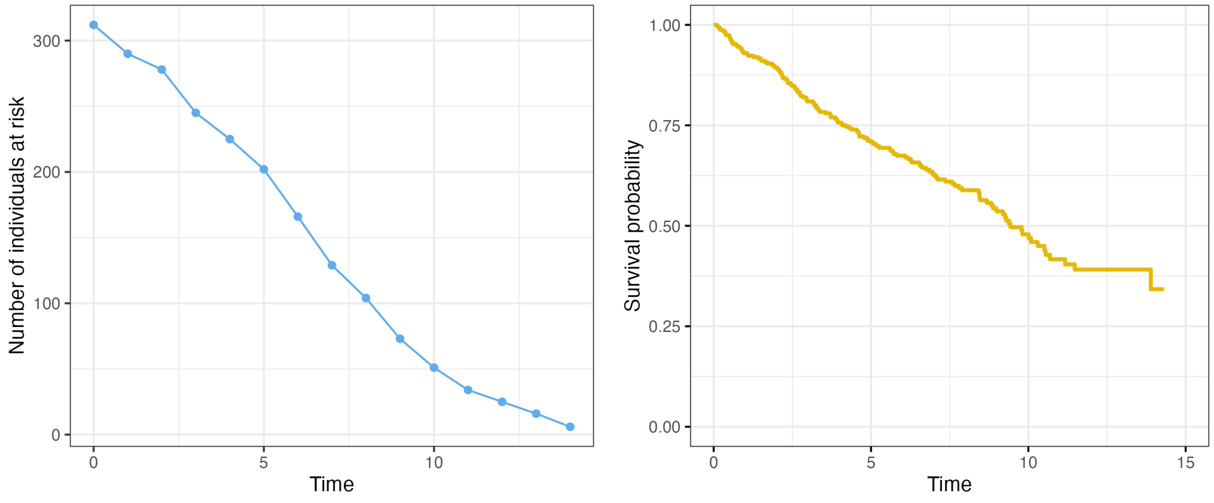


Figure 3: Number of subjects at risk (left) and Kaplan-Meier chart (right) for the PBC2 dataset.
